# Supplementary material for: First Measurement of Near- and Sub-Threshold $J/\psi$ Photoproduction off Nuclei
Source: arXiv:2409.18463 ancillary file (2024-10-23)
Supplement: Supplementary file 1 [file SRC_CT_JPsi_Supplementary.pdf]

# First Measurement of Near- and Sub-Threshold $J/\psi$ Photoproduction off Nuclei: Supplemental Material

## EXTENDED DATA

Figure 1 shows the light-cone proxy mass for each target separately, integrating over the full energy range.

Table I gives the total cross sections for helium, carbon, and the combined dataset in bins of beam energy, together with the statistical and systematic uncertainties for each bin. Table II lists the uncertainty on the normalization of the cross sections for each nucleus.

Figure 2 shows the differential cross section as a function of momentum-transfer $|t|$ separately in the sub-threshold energy region $7 < E_\gamma < 8.2$ GeV and the above-threshold energy region $8.2 < E_\gamma < 10.6$ GeV. Data are compared with plane-wave calculations as well as calculations assuming two models of virtuality-dependent modification described in the following section.

Figure 3 shows the tagged photon luminosity incident on each target, binned as a function of incoming photon energy.

## PLANE-WAVE CALCULATIONS

The quasi-elastic channel $(\gamma, J/\psi p)$ was simulated using a factorized cross section model in the Plane-Wave Impulse Approximation (PWIA):

$$\frac{d\sigma(\gamma A \to J/\psi p X)}{dt d^3\vec{p}_i dE_i} = v_{\gamma i} \cdot \frac{d\sigma}{dt}(\gamma p \to J/\psi p) \cdot S(p_i, E_i) \quad (1)$$

where $p_i = (E_i, \vec{p}_i)$ is the 4-momentum of the struck proton $i$ inside the nucleus, $p_\gamma$ is the 4-momentum of the incoming beam photon, $v_{\gamma i} = p_\gamma \cdot p_i/(E_\gamma E_i)$ is the relative velocity between the photon and the struck proton, $S(p_i, E_i)$ is the nuclear spectral function, and the differential cross section $d\sigma/dt$ for the exclusive process $(\gamma p \to J/\psi p)$ was taken from a fit to GlueX data [1]. This fit took the functional form for the total cross section following Refs. [2, 3]

$$\sigma_{\text{tot}} = \sigma_0 \cdot (1-\chi)^\beta \,, \quad (2)$$

where

$$\chi = \frac{m_{J/\psi}^2 + 2m_p m_{J/\psi}}{s_{\gamma p} - m_p^2} = \frac{E_\gamma^{th}}{E_\gamma} \quad (3)$$

is the so-called "energy fraction" parameter, $s_{\gamma p}$ is the squared center-of-mass energy of the photon-proton system, $m_p$ is the proton mass, $m_{J/\psi}$ is the $J/\psi$ mass, and

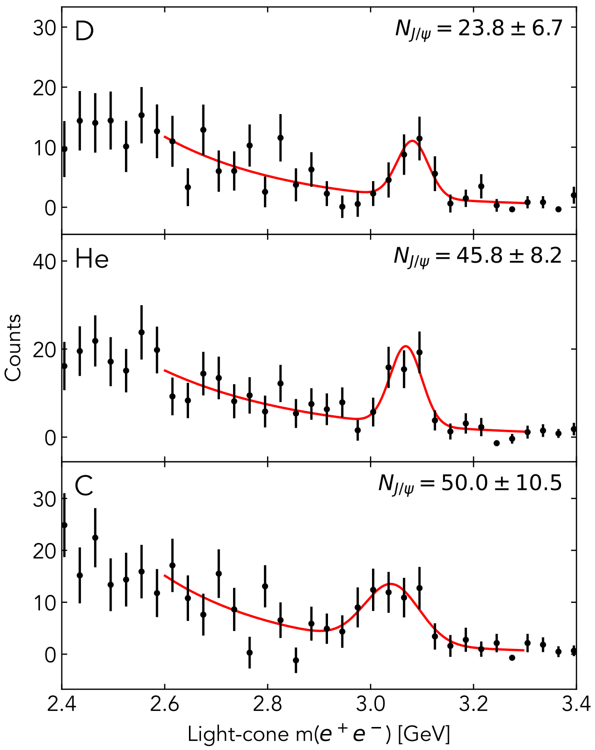


FIG. 1. Light-cone mass distributions for deuterium (top), helium (middle), and carbon (bottom) separately. Each distribution is fit with an exponential background model and a gaussian signal. In all cases the $J/\psi \to e^+e^-$ decays can be clearly observed.

TABLE I. Total cross sections for A$(\gamma, J/\psi p)X$ in bins of beam photon energy.

| Energy Bin | Nucleus | $\sigma(E)$ [nb] | Stat. [nb] | Sys. [nb] |
|---|---|---|---|---|
| 7-8.2 GeV | $^4$He | 0.17 | 0.08 | 0.05 |
| | $^{12}$C | 0.11 | 0.05 | 0.03 |
| | Combined | 0.14 | 0.05 | 0.04 |
| 8.2-9.5 GeV | $^4$He | 0.43 | 0.09 | 0.06 |
| | $^{12}$C | 0.16 | 0.06 | 0.04 |
| | Combined | 0.27 | 0.05 | 0.05 |
| 9.5-10.6 GeV | $^4$He | 0.50 | 0.15 | 0.09 |
| | $^{12}$C | 0.68 | 0.22 | 0.07 |
| | Combined | 0.61 | 0.15 | 0.08 |

TABLE II.

| Source of Uncertainty | Deuterium | Helium | Carbon |
|---|---|---|---|
| Luminosity | 0.54% | 0.32% | 0.07% |
| Efficiency | 19.5% | 19.5% | 19.5% |
| Transparency | 1% | 9% | 14% |
| Total | 20% | 21% | 24% |

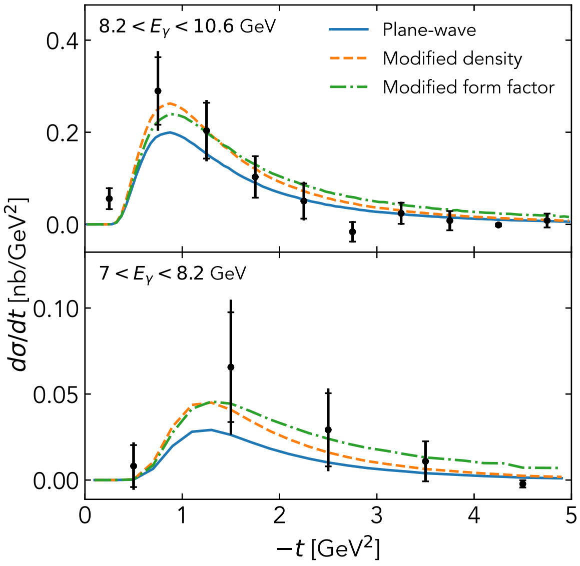


FIG. 2. Differential A$(\gamma, J/\psi p)X$ cross section as a function of momentum-transfer $t$, separated into the above-threshold (top) and below-threshold (bottom) energy regions. Measured data (black points) are compared with plane-wave calculations (blue solid line), as well as calculations assuming a modified proton density (orange dashed) and a modified form factor (green dot-dashed). Data also includes a common 23% normalization uncertainty (not shown).

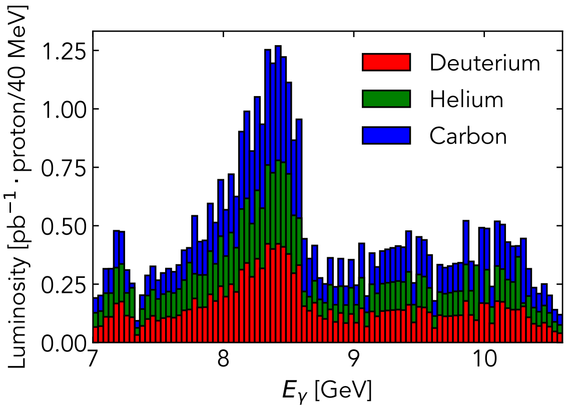


FIG. 3. Tagged luminosity for each target in bins of beam photon energy.

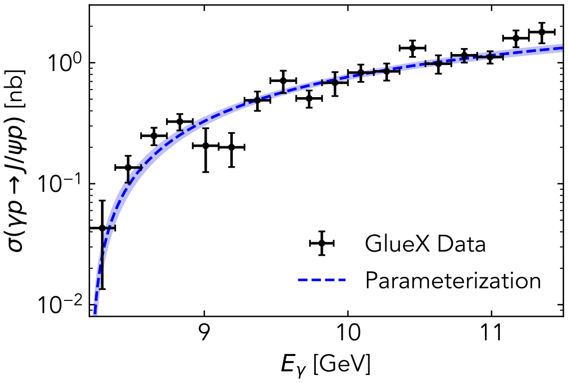


FIG. 4. Total $\gamma p \to J/\psi p$ cross section measurements of Ref. [1] (black) compared with analytic parameterization (blue) given in Equations 2 and 3.

the values $\sigma_0 = 5.9 \pm 1.0$ nb and $\beta = 1.2 \pm 0.1$ were found fitting to data, as shown in Fig. 4.

Because the Mandelstam variables are not uniquely defined in the case of off-shell initial-state particles, we choose to define the input values for the photon-nucleon cross section in terms of the momentum of the beam photon $p_\gamma$ and the final-state, positron $p_{e^+}$, electron $p_{e^-}$, and proton $p_p$:

$$s_{\gamma p} = (p_{e^+} + p_{e^-} + p_p)^2 \tag{4}$$

$$t = (p_\gamma - p_{e^+} - p_{e^-})^2 \,. \tag{5}$$

For the purposes of the plane-wave calculations, the photon-proton cross section was evaluated at these values of the Mandelstam variables. This means that the "effective" photon energy for the interaction must be calculated after accounting for the impact of motion within the nucleus:

$$k_{eff} \equiv \frac{s_{\gamma m} - m_p^2}{2m_p} \approx \alpha_i \cdot E_\gamma \tag{6}$$

where $\alpha_i = (E_i - p_{z,i})/(m_A/A)$ is the light-cone momentum fraction of the struck proton. In the plane-wave calculation we use the exact expression for $k_{eff}$ rather than using this approximation, which neglects the effects of proton virtuality.

The $t$-dependence of the cross section was assumed to follow a dipole form $F(t) \sim \frac{1}{(1-t/m_s^2)^2}$, using a weighted average $m_s = 1.35 \pm 0.04$ GeV for the dipole parameter following extractions in Ref. [1], assuming weak dependence on $s_{\gamma p}$. The differential cross section is related to the total cross section by the following:

$$\frac{d\sigma}{dt} = \sigma_{\rm tot} \frac{F^2(t)}{\int_{t_{\rm min}}^{t_{\rm max}} F^2(t) dt} \,. \tag{7}$$

The spectral functions for helium and carbon were taken from Ref. [4] for the mean-field component and the Generalized Contact Formalism [5–7] for the SRC component, calculated using the phenomenological AV18 interaction [8]. The momentum distribution for deuterium was taken from Ref. [9], again calculated using the AV18 interaction. The produced $J/\psi$ was assumed to conserve the helicity of the incoming photon, with the decay

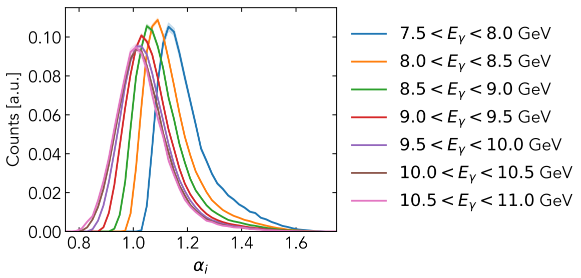


FIG. 5. The distribution of struck proton light-cone momentum fraction, $\alpha_i$, for different beam-photon energies, $E_\gamma$ in the rest frame of the nucleus. From simulated $\gamma^4$He$\to J/\psi pX$ events.

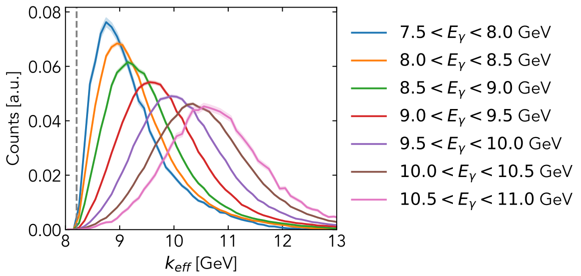


FIG. 6. "Effective" photon energy in simulated $\gamma^4$He$\to J/\psi pX$ events, binned as a function of the lab-frame beam-photon energy. The $\gamma p \to J/\psi p$ photon energy threshold is plotted at $E_\gamma^{th} \approx 8.2$ GeV as the grey dashed line. For events in the near- and sub-threshold region, the effective photon energy can be seen to deviate from the lab-frame energy as higher-momentum states become preferred.

following a $(1 + \cos^2\theta_{GJ})$ distribution in the Gottfried-Jackson frame.

Figure 5 shows the distribution of struck proton momentum-fraction $\alpha_i$ as a function of the beam-photon energy in the rest frame of the nucleus. We note that $\alpha_i \sim 1$ is the kinematics of a proton at rest within the nucleus, and is the most likely configuration at higher energies. $\alpha_i > 1$ represents a proton moving opposite the direction of the beam-photon; as this movement increases the center-of-mass energy of the photon-proton system and therefore the phase-space available for $J/\psi$ photoproduction, larger $\alpha_i$ is preferred in these near-threshold kinematics. As the beam photon energy is further reduced, the enhancement to large $\alpha_i$ becomes more pronounced as phase-space is more restricted. In the sub-threshold region of $E_\gamma < 8.2$ GeV, $\alpha_i > 1$ is kinematically required for $J/\psi$ photoproduction.

Figure 6 shows the "effective" beam photon energy $k_{eff}$ as a function of the lab-frame photon energy $E_\gamma$. The effective photon energy is distorted by the motion of the proton by an approximate factor of $\alpha_i$. As such, the effective photon energy differs significantly from the lab-frame photon energy in all kinematics. At higher energies, the impact of nuclear motion is largely symmetric, both increasing and decreasing the effective photon momentum. At lower energies, near and below the threshold, the proximity of the threshold energy $E_\gamma^{th} \approx 8.2$, or correspondingly a lack of phase-space for the photoproduction of $J/\psi$ from the proton, forces an increase in the light-cone momentum fraction and therefore the effective photon energy. We observe here that, even in the sub-threshold region $E_\gamma < 8.2$ GeV, the effective photon energy has a very wide distribution, averaging greater than 9 GeV, and is not strongly dependent on the immediate threshold behavior of the $\gamma p \to J/\psi p$ interaction.

The virtuality of the struck proton is defined as

$$v = (p_i^2 - m_N^2)/m_N^2 < 0\,, \tag{8}$$

where $p_i = (E_i, \vec{p}_i)$ is the off-shell 4-momentum of the proton, and quantifies the binding of the proton inside the nucleus. The "density modification" hypothesis considered the possibility that the photon-proton cross section scaled with increasing $|v|$:

$$\frac{d\sigma}{dt} \to (1 - av) \times \left.\frac{d\sigma}{dt}\right|_{\text{free}}\,, \tag{9}$$

where $a = 2$ was the data's best-fit value. The "form factor modification" hypothesis considered the possibility that the dipole mass parameter increases with increasing $|v|$:

$$m_s \to m_{s,\text{free}}/(1 + bv)\,, \tag{10}$$

where $b = 0.4$ was the data's best-fit value.

## PROTON TRANSPARENCY

As the final state measured in this reaction includes both the $J/\psi \to e^+e^-$ decay and the knocked-out proton, the effects of nuclear transparency must be considered. For the $J/\psi$, this effect can be neglected because even in the case of rescattering, the leptonic decay will still be detected and overall yields will be unaffected. For the proton, the transparency factor must be accounted for in determining the cross section.

In the case of deuterium, measurements of $(e, e'p)$ quasi-elastic scattering [10, 11] may be used to determine a data-driven estimate of $90 \pm 1\%$ transparency on protons at $\mathcal{O}(1\text{ GeV})$ momentum, with little deviation as a function of momentum.

For helium and carbon, proton transparency was calculated using a Glauber model as used in Ref. [12]. The transparency for a proton in the nucleus is given by the equation

$$T = \frac{1}{A}\int d^3r\rho(r)\exp\left(-\sigma_{\text{eff}}\int dl\hat{z}\rho(r)\right)\,, \tag{11}$$

where $\rho(r)$ is the position-space nuclear density and $\sigma_{\text{eff}}$ is the effective proton cross section in the nuclear medium. The nuclear densities were taken from Ref. [13]. The effective proton cross sections were taken from Ref. [11] for proton momentum greater than 900 MeV/$c$ and from Ref. [14] for lower proton momentum.

This model gives a transparency of $64.8 \pm 7.1\%$ for helium and $58.0 \pm 8.4$ for carbon, where the transparency is taken for the average proton momentum in signal Monte-Carlo.

## LIGHT-CONE MASS PROXY

In exclusive $\gamma p \to e^+e^-p$ events, the invariant dilepton mass $m^2(e^+e^-)$ is well-reconstructed, as kinematically fitting the event with the requirement of full 4-momentum conservation leads to well-reconstructed lepton momentum. With nuclear targets and non-exclusive $\gamma A \to e^+e^-p(X)$ events, such restrictive kinematic fitting is not possible, and the resulting lepton momenta are more poorly reconstructed. This leads to a similarly poor reconstruction for the dilepton mass.

We note that with GlueX not all components of momentum are reconstructed equally well. In the solenoid magnetic field, the transverse component of momentum $\vec{p}_\perp$ can be reconstructed with good precision from the curvature of the tracks in the drift chambers. The longitudinal component $p_z$ and the energy $E$ are more poorly reconstructed, requiring a combination of the longitudinal momentum component and the polar angle $\theta$ of the track. The use of "light front" variable can help to mitigate these challenges. The energy and longitudinal momentum can be expressed in two linear combinations, denoted the "plus" and "minus" components of momentum:

$$p^\pm = E \pm p_z \,. \tag{12}$$

It is helpful also to note the momentum-mass relation in terms of these components:

$$m^2 = p^+p^- - p_\perp^2 \,. \tag{13}$$

These variables have previously been used in analysis of nucleon knockout data with poor momentum resolution [15]. While the "plus" component of momentum is still poorly reconstructed, the "minus" component, representing the difference between the energy and longitudinal momentum, suffers very little smearing as a result of detector resolution:

$$\frac{\partial p^-}{\partial p_z} = \frac{p_z}{E} - 1 = \mathcal{O}\left(p_\perp^2/p_z^2\right) \,. \tag{14}$$

This effect, combined with the relatively small smearing for the transverse components of momentum in GlueX (a consequence of the solenoid magnet), provides us a combination of momentum variables that may be reliably used to describe the initial nuclear state. We note that for the final-state proton, which is low momentum, the impact of smearing is relatively small in reconstructed variables; for the high-momentum final-state leptons, this smearing is much larger, and thus the plus components of the lepton momentum $p^+_{e^\pm}$ are the most affected.

We may make the approximation that the scattering is performed from a standing pair of nucleons, with the recoil 4-momentum being carried by a single spectator nucleon. This gives us three equations defining conservation of 4-momentum:

$$p_{\gamma,\perp} + p_{2N,\perp} = 0 = p_{N,\perp} + p_{tot,\perp} \tag{15}$$
$$p_\gamma^- + p_{2N}^- = E_\gamma - E_\gamma + 2m_N = p_N^- + p_{tot}^- \tag{16}$$
$$p_\gamma^+ + p_{2N}^+ = E_\gamma + E_\gamma + 2m_N = p_N^+ + p_{tot}^+ \tag{17}$$

where $p_N$ is the 4-momentum of the spectator nucleon, and $p_{tot} = p_{e^+} + p_{e^-} + p_p$ is the momentum of the measured final-state.

The transverse momentum carried by this nucleon must be opposite the transverse momentum of the measured dilepton-proton system:

$$p_{N,\perp} = -p_{\text{tot},\perp} \,. \tag{18}$$

The minus component of momentum is also given by conservation of 4-momentum:

$$p_N^- = 2m_N - p_{\text{tot}}^- \,. \tag{19}$$

The plus component of momentum can be calculated using the assumed mass of the spectator:

$$p_N^+ = \frac{m_N^2 + p_{N,\perp}^2}{p_N^-} = \frac{m_N^2 + p_{tot,\perp}^2}{2m_N - p_{\text{tot}}^-} \,. \tag{20}$$

Conservation of 4-momentum again allows us to connect the plus component of the dilepton system with that of the proton, the beam, the standing pair, and the assumed spectator:

$$p_{e^+}^+ + p_{e^-}^+ = 2E_\gamma + 2m_N - p_p^+ - p_N^+ \,. \tag{21}$$

Combining these equations, we may construct our "light-cone" mass proxy variable:

$$\begin{aligned} m^2(e^+e^-) &\approx m^2_{\text{light-cone}} \\ &= \left(p_{e^+}^- + p_{e^-}^-\right)\left(2E_\gamma + 2m_N - p_p^+ - \frac{m_N^2 + p_{\text{tot}}^2}{2m_N - p_{\text{tot}}^-}\right) \\ &\quad - \left(\vec{p}_{e^+}^{\perp} + \vec{p}_{e^-}^{\perp}\right)^2 \,. \end{aligned} \tag{22}$$

We present in Figure 7 the impact of our standing pair assumption on a "two-nucleon missing mass":

$$m^2_{\text{miss},2N} = \left(p_\gamma + p_{2N} - p_{e^+} - p_{e^-} - p_p\right)^2 \,, \tag{23}$$

and the reconstructed dilepton mass. The light-cone mass proxy can be seen to have improved resolution over the reconstructed invariant mass by over a factor of 2, enabling identification of the $J/\psi \to e^+e^-$ decay over backgrounds.

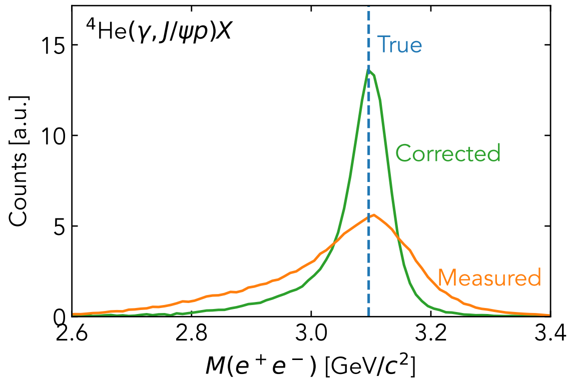


FIG. 7. Dilepton invariant mass (orange), compared with the corrected "lightcone" mass using the 2N-breakup assumption (green) in simulated $J/\psi$ production from helium. Also shown is the true $J/\psi$ mass of 3.096 GeV/$c^2$ (blue). The corrected observable shows significantly improved resolution compared with the regular invariant mass.

Figure 8 displays the correlation between the $J/\psi$ reconstructed mass and the kinematic variables $t$, $\alpha_{miss}$, and missing $p_T$, using both the dilepton invariant mass and the light-cone mass in simulated events from $^4$He. We observe that the light-cone mass has both substantially improved resolution and far less kinematic dependence than the measured mass for the dilepton system, resulting in both increased precision and decreased model-dependence in the extracted differential cross sections.

We observe that in Figure 1, the extracted mass is slightly shifted between targets, being $3.082 \pm 0.010$ GeV/$c^2$ for deuterium, $3.069 \pm 0.006$ GeV/$c^2$ for helium, and $3.041 \pm 0.010$ GeV/$c^2$ for carbon. As the light-cone mass proxy requires measurement not only of the leptons but of the proton, it can be sensitive to proton rescattering as well as effects which impact the lepton momentum. Figure 9 shows the impact of simplistic final-state rescattering of either the $J/\psi$ or the proton in the nucleus on the light-cone mass, without including the impact of detector smearing. The cases were considered where the particle lost 5% of its momentum, and where the angle of the particle was smeared by a width of 5°. It is seen that the rescattering of these final-state particles can impact the reconstructed light-cone mass, though more detailed FSI calculations would be necessary to match the mass shifts observed in the data.


[1] S. Adhikari *et al.* (GlueX Collaboration), Measurement of the $J/\psi$ photoproduction cross section over the full near-threshold kinematic region, Phys. Rev. C **108**, 025201 (2023).
[2] J. Xu and F. Yuan, Gluonic probe for the short range correlation in nucleus, Physics Letters B **801**, 135187 (2020).
[3] Y. Hatta *et al.*, Sub-threshold J/$\psi$ and $\Upsilon$ production in $\gamma$A collisions, Physics Letters B **803**, 135321 (2020).
[4] N. Rocco and A. Lovato, private communication.
[5] R. Weiss *et al.*, Energy and momentum dependence of nuclear short-range correlations - Spectral function, exclusive scattering experiments and the contact formalism, Phys. Lett. **B791**, 242 (2019), arXiv:1806.10217 [nucl-th].
[6] A. Schmidt *et al.* (CLAS), Probing the core of the strong nuclear interaction, Nature **578**, 540 (2020), arXiv:2004.11221 [nucl-ex].
[7] J. Pybus *et al.*, Generalized contact formalism analysis of the $^4$He$(e, e'pN)$ reaction, Phys. Lett. B **805**, 135429 (2020), arXiv:2003.02318 [nucl-th].
[8] S. Veerasamy and W. N. Polyzou, Momentum-space Argonne V18 interaction, Phys. Rev. C **84**, 034003 (2011).
[9] R. B. Wiringa *et al.*, Nucleon and nucleon-pair momentum distributions in $A \leq 12$, Phys. Rev. C **89**, 024305 (2014).
[10] D. Abbott *et al.*, Quasifree $(e, e'p)$ reactions and proton propagation in nuclei, Phys. Rev. Lett. **80**, 5072 (1998).
[11] K. Garrow and et. al., Nuclear transparency from quasielastic a(e,e'p) reactions up to qsup 2=8.1 (gev/c)sup 2, Physical Review C **66**, 10.1103/PhysRevC.66.044613 (2001).
[12] O. Hen *et al.*, Momentum sharing in imbalanced Fermi systems, Science **346**, 614 (2014), arXiv:1412.0138 [nucl-ex].
[13] H. De Vries *et al.*, Nuclear charge-density-distribution parameters from elastic electron scattering, Atomic Data and Nuclear Data Tables **36**, 495 (1987).
[14] V. R. Pandharipande and S. C. Pieper, Nuclear transparency to intermediate-energy nucleons from (e,e'p) reactions, Phys. Rev. C **45**, 791 (1992).
[15] E. Piasetzky *et al.*, Evidence for the strong dominance of proton-neutron correlations in nuclei, Phys. Rev. Lett. **97**, 162504 (2006), arXiv:nucl-th/0604012 [nucl-th].

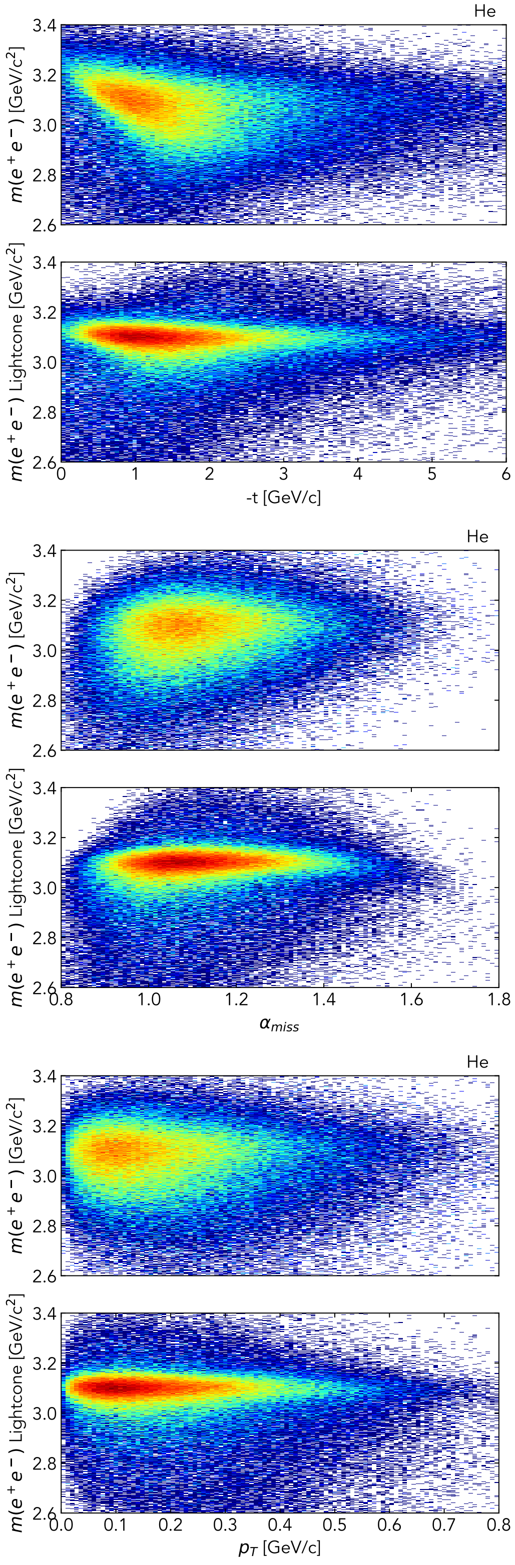


FIG. 8. Correlation between the $J/\psi$ reconstructed mass and the kinematic variables $t$, $\alpha_{miss}$, and missing $p_T$. Correlation is shown for both the measured dilepton mass and the light-cone mass in simulated events from $^4$He.

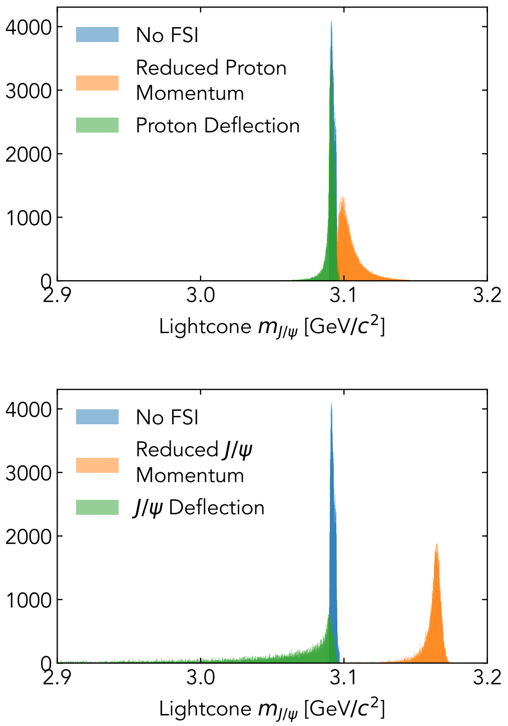


FIG. 9. *Top:* The impact of proton FSI on the light-cone $J/\psi$ momentum, including a 5% reduction in the proton momentum and a $\sigma_\theta = 5^\circ$ smearing of the proton angle. *Bottom:* The impact of the same FSI applied to the $J/\psi$ momentum.
